# Supplementary material for: The wave equation on subextremal Kerr spacetimes with small non-decaying first order terms
Source: arXiv:2302.06387 source file (2023-02-13)
Supplement: Supplementary file 1 [file CommutatorBoundsAppendix.tex]

%Here we prove Theorem \ref{thm:WProperties}, as well as certain technical results which appear in the same section. In order to keep the flow of the argument clear, all statements made in Sections \ref{sec:freunique} and \ref{sec:fPrimeBounds} are written in a manner independently of the choices of the regimes $\mathcal{G}, \mathcal{G}'$, as the choice of constants $\ximin, \ximax$ which determine these regimes depend on the constant $c_0$ appearing in Proposition \ref{lem:fprimelowerbound}. We define the set 
%\begin{equation}
%\mathcal{G}'_{max} = \left\{(\omega, m) \in \mathbb{R}\times\mathbb{Z} \,|\, \omega \neq 0 \text{ and }m\omega\notin (0, m\omega_+]\right\}.
%\end{equation}
%It follows that $\mathcal{G}'\subset\mathcal{G}'_{max}$ excluding $(0,0)$. All results in Sections \ref{sec:freunique} and \ref{sec:fPrimeBounds} are proven for $(\omega, m)\in\mathcal{G}'_{max}$, from which results for $\mathcal{G}'$ directly follow.

%For $(\omega, m)\in\mathcal{G}'_{max}$, we recall from \eqref{def:fsquaredabstract} and \eqref{def:fsquaredconstantterm} that $\f$ given in \eqref{def:f2} is uniquely defined only if
%\begin{equation}\label{id:fsquareddef}
%\f^2 = \frac{(\omega-\omega_r)^2}{\omega^2v^2} - \inf\frac{(\omega-\omega_r)^2}{\omega^2v^2}.%= \frac{(\omega-\omega_r)^2}{\omega^2v^2} - C\left(\frac{m}{\omega}\right).
%\end{equation}
%has a unique minimum at $\re \in (r_+, \infty)$. Before we prove this, we define certain quantities which we will use throughout this section.

%For $\omega \neq 0$, and assuming as usual $a>0$, we recall
%\begin{equation}
%\eta = \frac{am}{\omega},
%\end{equation}
%defined in \eqref{def:eta}, noting that all quantities which may be written as functions of $\eta, r$ are homogeneous of degree 0 in $(\omega, m)$.
% We additionally define
%\begin{equation}
%\Gamma = \Gamma(r, \eta)\index{Gamma@$\Gamma$} = (r^2+a^2)\tfrac{\omega-\omega_r}{\omega} = r^2 + a^2 - \eta,  \qquad \Gamma_+\index{GammaPlus@$\Gamma_+$} = \Gamma(r_+, \eta).
%\end{equation}
%As with $\Delta$, we suppress dependence of $\Gamma$ on $r$, as well as on $\eta$. For $(\omega, m) \in \mathcal{G}'_{max}$, it follows from straightforward calculation that



%\subsection{Proof of statement (\ref{Thm:flowerbound}) of Theorem \ref{thm:WProperties}}
%The following Lemma easily implies the desired statement and moreover establishes an explicit constant for the required coercivity:
%\begin{lemma}\label{lem:fprimelowerbound}
%Let $(\omega, m)$ be such that both $\omega \neq 0$ and $m\omega \notin (0, m\omega_+]$. The function $\f$ defined in \eqref{def:f2} obeys the inequality
%\begin{equation}\label{est:fprimelowerbound}
%v\Rs\f \geq \tfrac{c_0}{r}\tfrac{\omega-\omega_r}{\omega},
%\end{equation}
%where 
%\begin{equation}\index{cnatural@$c_0$}
%c_0 = \frac12\left(\tfrac{r_+-M}{r_+}\right)^3 \, .
%\end{equation}
%\end{lemma}



%We now prove a series of  estimates on the trapping radius and the commutator function $\f$, which will be used in Section \ref{sec:CEE} and Appendix \ref{sec:CMConvolution}. Since $\ximin, \ximax$ have been fixed at that point, as such, bounds appearing here may depend on $\ximin, \ximax$ without issue. 


%\subsection{Proof of statement (\ref{Thm:Plupperbound}) of Theorem \ref{thm:WProperties}} %{Bounds on lower order commutator terms}

%We now seek to bound $\Pl$. Recalling the definition \eqref{def:fetaTrue}, we construct this via bounds on individual components. We first take a technical proposition which will simplify calculations on $\ve$.

%We repeat the desired statement as the following proposition:
%\begin{proposition}\label{prop:PlBound}
%Given $\Pl^\natural$ as defined in \eqref{def:Pl}, we have the estimate
%\begin{equation}\label{est:PlBound}
%|\Pl^\natural\ph|\leq C\left( r^{-3}|\Wsv\ph| +  v^{3}(|\omega\ph| + |\ph|)\right),
%\end{equation}
%for a constant $C$ depending only on $M$, $a$, $\ximin$, and $\ximax$.
%\end{proposition}
%\begin{proof}
%\end{proof}
