# Supplementary material for: The wave equation on subextremal Kerr spacetimes with small non-decaying first order terms
Source: arXiv:2302.06387 source file (2023-02-13)
Supplement: Supplementary file 2 [file InhomogeneousAppendix.tex]

In section \ref{sec:LOT} we extended results on the homogeneous wave equation to the perturbed wave equation. As our extension required slight but straightforward adaptations of several technical results, we have postponed the proof of those lemmas until now. We remark that in this chapter we will introduce notation from cited papers.
\subsection{Establishing future integrability}
Here we restate the conditions of future integrability and outgoing boundary conditions from \cite{DRSR}, and verify that the weakened conditions present here remain sufficient to establish the outgoing boundary conditions for the frequency-separated equations.  We say a function is \emph{future integrable} if
\begin{equation}
\int...
\end{equation}
A function satisfies the \emph{outgoing boundary conditions} if
\begin{equation}
\lim ...
\end{equation}

\subsubsection{The horizon estimate for non-stationary bounded frequencies}\label{sec:fluxestimates} In order to make full use of Theorem \ref{thm:DRSRMain}, we must show a horizon estimate for non-stationary bounded frequencies which is analogous to the results of the standard wave equation given in \cite{SR14}. 
\begin{lemma}
Given a function $\Psi_T$ solving the equation \eqref{def:PhysCutoffEq},
Theorem 1.9 of \cite{SR14} holds with the following modification:
\begin{align}
\int_{\mathcal{H}^+}&|\mathcal{P}_{\mathcal{B}, \mathcal{C}}\Psi_\chi|^2 + \int_{\mathcal{I}^+}|\partial\mathcal{P}_{\mathcal{B}, \mathcal{C}}\Psi_\chi|^2 + \int_{\mathbb{R}\times (r_0, r_1)\times \mathbb{S}^2}|\mathcal{P}_{\mathcal{B}, \mathcal{C}}\Psi_\chi|^2 \\
&\leq B(r_0, r_1, C_{\mathcal{B}}, C_{\mathcal{C}}, a, M)\left(\int_{\widetilde{\Sigma}_0}|\partial\Psi_T|^2+ \varepsilon\mathcal{S}[\Psi_\chi]\right) 
\end{align}
\end{lemma}
The proof closely follows section 3 in \cite{SR14}, so here we detail only additional considerations which arise from the perturbative term. In particular, we may reduce this to proving analogues to Lemmas 3.2 and 3.3 in the aforementioned work, as the results for the remainder of the section do not depend on the specific nature of the inhomogeneities. We first define, for $\epsilon \geq 0$,
\begin{equation}
\Psi_{T, \epsilon} = e^{-\epsilon t}\Psi_T,
\end{equation}
remarking that this serves the same purpose as $\psi_{\epsilon, \text{\LeftScissors}}$ in the aforementioned work. 
 First we replace the right hand side of the wave equation with that of the perturbed equation; i.e. \eqref{def:WaveEqCutoff}, to define
\begin{align}
E_\epsilon = e^{-\epsilon t}\big(\varepsilon\chi_T(\BfB \Psi_{\chi , T}) + 2\nabla^\alpha \chi \nabla_\alpha \Psi_T + (\Box_{g_{a, M}}\chi)\Psi_T - \varepsilon \chi_T\Psi_T (\BfB \chi)\big)
\end{align}
We define $F_\epsilon$, $H_\epsilon$ as in \cite{SR14}, based on our modified $E_\epsilon$. Proposition \ref{prop:suffi} implies exponential decay for $\Psi_{T, \epsilon}$ in $t$. This combined with decay of $\BfB$ in space implies exponential decay for $H_\epsilon$ in $\rs$. Therefore, the representation formula Proposition 3.1 of \cite{SR14} continues to hold.

In order to extend this representation formula to the $\epsilon = 0$ case, we adapt Lemma 3.2 from \cite{SR14}, noting that we need to add a spacetime term on the right hand side.
\begin{proposition}
Lemma 3.2 of \cite{SR14} holds under the following modification:
\begin{equation}
\limsup_{\epsilon\to 0^+}\int_{\mathcal{B}}\sum_{m, l}\int_{r_+}^\infty |F_\epsilon|^2 r^2\, dr\, d\omega = \int_{\mathcal{B}}\sum_{m, l}\int_{r_+}^\infty |F|^2 r^2\, dr\, d\omega \lesssim \int_{\Sigma_0}|\partial\psi|^2 + \varepsilon^2\mathcal{S}[\ph]
\end{equation}
\end{proposition}
\begin{proof}
The first equality follows from Plancherel's theorem along with the dominated convergence theorem, following from the future integrability condition. The inequality on the right follows from the decomposition \eqref{def:WavePerturbedFreq}. Then, terms appearing in $\Hchi$ may be be bounded as in \cite{SR14}, noting that $\BfB\chi$ generally decays faster than $\Box_{g_{a, M}}\chi$ in $r$. The result for $\HB$ follows from direct integration along with the Cauchy-Schwartz inequality.
\end{proof}
Adapting the integral for large $r$ is only slightly more involved, as we may no longer take advantage of compact support for $H$ in the $t-r$ variable. Fortunately, we may decompose $H$ into a term for which this holds and a term which is $L^1$ in the radial variable.
\begin{lemma}
Lemma 3.3 of \cite{SR14} holds with the following modification:
\begin{equation}
\left\lVert\int_{\rs}^\infty u_{out}(x^\star)H(x^\star)\, dx^\star\right\rVert_{L^2_{\omega\in\mathcal{B}. (m, \ell)\in\mathcal{C}}}^2\leq B(\rs, C_{\mathcal{B}}, C_{\mathcal{C}})\left(\int_{\Sigma_0}|\partial\Psi|^2 + \varepsilon^2\mathcal{S}[\ph]\right).
\end{equation}
and 
\begin{equation}
\lim_{\epsilon\to 0}\int_{\rs}^\infty u_{out, \epsilon}(x^\star)H_\epsilon(x^\star) \, dx^\star = \int_{\rs}^\infty u_{out}(x^\star)H(x^\star)\, dx^\star
\end{equation}
in $L^2_{\omega \in \mathcal{B}, (m, \ell)\in\mathcal{C}}$.
\end{lemma}
\begin{proof}
As in \cite{SR14} we may replace $u_{out}$ with its highest order part, and reduce this to Parseval's inequality in $x^\star$. We write
\begin{equation}
|u_{out}(\rs) - e^{i\omega \rs}|\leq Cr^{-1}
\end{equation}
and bound the terms with $r^{-1}$ decay as before. It suffices to prove the bound
\begin{equation}
\int_{\mathcal{B}}\sum_{m, \ell\in\mathcal{C}}\left|\int_{\rs}^\infty e^{i\omega x^\star}H(x^\star)\, dx^\star\right|^2 \, d\omega\leq B(\rs, C_{\mathcal{B}}, C_{\mathcal{C}})\left(\int_{\Sigma_0}|\partial\Psi|^2 + \varepsilon^2\mathcal{S}[\ph]\right)
\end{equation}
We again split $H$ as in \eqref{def:WavePerturbedFreq}, additionally decomposing in the spheroidal harmonics, and note that the theorem for $H_\chi$ follows as in \cite{SR14}, noting again that $\BfB\chi$ satisfies better decay bounds than $\Box_{g_{a, M}}\chi$ in $r$. To bound $H_\BfB$ terms, we note that H\"older's inequality implies
\begin{equation}
\left|\int_{\rs}^\infty e^{i\omega x^\star}H_\BfB(x^\star)\, dx^\star\right| \leq \left\lVert \Delta^{-1/2} r^{3/2+\alpha} H_\BfB \right\rVert_{L^2_{\rs}}\left\lVert \Delta^{1/2}r^{-3/2-\alpha}\right\rVert_{L^2_{\rs}}.
\end{equation}
Plancherel's theorem and direct integration imply
\begin{equation}
\int_{\mathcal{B}}\sum_{m, \ell\in\mathcal{C}}\left\lVert \Delta^{-1/2} r^{3/2+\alpha} H_\BfB \right\rVert_{L^2_{\rs}} \lesssim \varepsilon^2\mathcal{S}[\ph], \qquad \left\lVert \Delta^{1/2}r^{-3/2-\alpha}\right\rVert_{L^2_{\rs}} \lesssim C_\alpha.
\end{equation}
The remainder of the proof follows as in \cite{SR14}.
\end{proof}
To conclude, we restate this proposition in a way which will apply to Section \ref{sec:LOT}:
\begin{proposition}
Let $\mathcal{B}\subset\mathbb{R}$ and let $\mathcal{C} \subset \{(m, \ell) \in \mathbb{Z}\times\mathbb{Z} : \ell \geq |m|\}$ such that
\begin{equation}
\sup_{\omega \in \mathcal{B}, (m, \ell)\in\mathcal{C}} |\omega|+|\omega^{-1}|+|m|+|\ell| \leq \infty. 
\end{equation}
Then, there exists a constant $ C_{\mathcal{B}, \mathcal{C}}$ depending on $\mathcal{B}, \mathcal{C}$ such that
\begin{equation}
\int_{\mathcal{B}}\sum_{m, \ell\in\mathcal{C}} |\uchi(-\infty)|^2\leq  C_{\mathcal{B}, \mathcal{C}}\left(E_0[\Psi]+\mathcal{S}[\uchi]\right).
\end{equation}
\end{proposition}
